# Supplementary material for: At the same age, metallicity, and alpha-enhancement, sodium is a more effective tracer of the young and old sequences of the Milky Way disc
Source: arXiv:2405.00315 source file (2024-10-13)
Supplement: Supplementary file 1 [file slope_5.0_6.5_Si.tex]

$0.0053 \pm 0.0035\,\mathrm{dex/Gyr}$
