# Supplementary material for: At the same age, metallicity, and alpha-enhancement, sodium is a more effective tracer of the young and old sequences of the Milky Way disc
Source: arXiv:2405.00315 source file (2024-10-13)
Supplement: Supplementary file 3 [file slope_6.5_8.0_Si.tex]

$-0.0068 \pm 0.0024\,\mathrm{dex/Gyr}$
